# Supplementary material for: Search for a high-mass Higgs boson decaying to a $W$ boson pair in $pp$ collisions at $\sqrt{s} = 8$ TeV with the ATLAS detector
Source: arXiv:1509.00389 source file (2016-01-18)
Supplement: Supplementary file 1 [file appendix.tex]

\section{Two-Higgs-Doublet Model}

\subsection{Modelling of input variables}

\begin{figure*}[!h] 
 \centering 
 \subfloat[]{
  \includegraphics[width=0.45\textwidth]{fig/NN/Mjj_Stacked_NormDat_selection_165_195_topCR.png}
 }
 \subfloat[]{
  \includegraphics[width=0.45\textwidth]{fig/NN/Mll_Stacked_NormDat_selection_165_195_topCR.png}
 }

 \vspace*{2mm}

 \subfloat[]{
  \includegraphics[width=0.45\textwidth]{fig/NN/MT_Stacked_NormDat_selection_165_195_topCR.png}
 } 
 \subfloat[]{
  \includegraphics[width=0.45\textwidth]{fig/NN/j1pt_Stacked_NormDat_selection_165_195_topCR.png}
 }

 \caption{Examples of distributions of four important input va\-ri\-ables in the 
         2-jet channel in the $b$-tagged control region using selection cuts applied
         in the mass region 165 -- 195 GeV.
         The distributions of simulated events are normalised to the number of observed 
         events in data.}
 \label{fig:CR_top_mh180}
\end{figure*}

\begin{figure*}[p] 
 \centering 
 \subfloat[]{
  \includegraphics[width=0.45\textwidth]{fig/NN/Mll_Stacked_NormBillFit_jb0.png}
 }
 \subfloat[]{
  \includegraphics[width=0.45\textwidth]{fig/NN/lldPt_Stacked_NormBillFit_jb0.png}
 }

 \vspace*{2mm}

 \subfloat[]{
  \includegraphics[width=0.45\textwidth]{fig/NN/MT_Stacked_NormBillFit_jb1.png}
 }
 \subfloat[]{
  \includegraphics[width=0.45\textwidth]{fig/NN/DPhiMETlep1_Stacked_NormBillFit_jb1.png}
 } 

 \caption{Examples of distributions of important input va\-ri\-ables for the 2HDM search analysis 
  in the 0-jet channel in the light Higgs region.
  The distributions of simulated events are normalised to the fit results obtained when fitting
  the NN discriminant light Higgs region for normalisation purposes only.}
 \label{fig:lightHiggs_input}
 \end{figure*}

\clearpage
\subsection{Shapes of NN discriminants}

\begin{figure*}[!h]
 \centering
 \subfloat[][$m_{\rm H}=240$~GeV, 0 jets]{
  \includegraphics[width=0.32\textwidth]{fig/NN/NNout_Shapes_mh240_jb0.png}
 }
 \subfloat[][$m_{\rm H}=240$~GeV, 1 jet]{
  \includegraphics[width=0.32\textwidth]{fig/NN/NNout_Shapes_mh240_jb1.png}
 }
 \subfloat[][$m_{\rm H}=240$~GeV, 2 jets]{
  \includegraphics[width=0.32\textwidth]{fig/NN/NNout_Shapes_mh240_jb2.png}
 }
  
 \vspace*{4mm}

 \subfloat[][$m_{\rm H}=400$~GeV, 0 jets]{
  \includegraphics[width=0.32\textwidth]{fig/NN/NNout_Shapes_mh400_jb0.png}
 }
 \subfloat[][$m_{\rm H}=400$~GeV, 1 jet]{
  \includegraphics[width=0.32\textwidth]{fig/NN/NNout_Shapes_mh400_jb1.png}
 }
 \subfloat[][$m_{\rm H}=400$~GeV, 2 jets]{
  \includegraphics[width=0.32\textwidth]{fig/NN/NNout_Shapes_mh400_jb2.png}
 }
  
 \vspace*{4mm}

 \subfloat[][$m_{\rm H}=600$~GeV, 0 jets]{
  \includegraphics[width=0.32\textwidth]{fig/NN/NNout_Shapes_mh600_jb0.png}
 }
 \subfloat[][$m_{\rm H}=600$~GeV, 1 jet]{
  \includegraphics[width=0.32\textwidth]{fig/NN/NNout_Shapes_mh600_jb1.png}
 }
 \subfloat[][$m_{\rm H}=600$~GeV, 2 jets]{
  \includegraphics[width=0.32\textwidth]{fig/NN/NNout_Shapes_mh600_jb2.png}
 }
  
 \caption{Output distributions of the neural networks for three different Higgs
  mass points in the signal region as shape plot 
  (on the left for the 0 jet channel, in the centre for the 1-jet channel and on 
  the right for the 2-jet channel). The heavy Higgs signal is split into 
  gluon-gluon fusion (dark red) and VBF (light red) contributions. 
  The background processes are summed up to show the discrimination power of the neural 
  network.}
  \label{fig:NNout_Shapes_w2HDM}
\end{figure*}

\clearpage
\subsection{Post-fit NN discriminant distributions}

\begin{figure*}[!h] 
 \centering 
 \subfloat[]{
  \includegraphics[width=0.45\textwidth]{fig/NN/NNout_Stacked_NormBillFit_lowMass_CR_jb0.png}
 }
 \subfloat[]{
   \includegraphics[width=0.45\textwidth]{fig/NN/NNout_Stacked_NormBillFit_lowMass_CR_jb1.png}
 }
\caption{NN output distributions of the light Higgs region. (a) shows the NN discriminant 
 distribution the 0-jet channel and (b) the distribution of the 1-jet channel. 
 The distributions of simulated events are normalised to the fit values.}
% given in table~\ref{tab:lightHiggsFitValues}.}
 \label{fig:NNout_lightHiggsRegion}
\end{figure*}

\begin{figure*}[!h] 
 \centering 
 \subfloat[]{
  \includegraphics[width=0.32\textwidth]{fig/NN/NNout_Stacked_NormBillFit_mh150_jb0.png}
 }
 \subfloat[]{
  \includegraphics[width=0.32\textwidth]{fig/NN/NNout_Stacked_NormBillFit_mh150_jb1.png}
 }
 \subfloat[]{
  \includegraphics[width=0.32\textwidth]{fig/NN/NNout_Stacked_NormBillFit_mh150_jb2.png}
 }
\caption{NN output distributions of the signal region in the 135 -- 160 GeV mass region , 
 for which the NN was trained at 150 GeV. The subfigure (a) shows the NN discriminant distribution 
 in the 0-jet channel, (b) the distribution of the 1-jet channel and 
 (c) the distribution of the 2-jet channel. 
 The distributions of simulated events are normalised to data.}
 \label{fig:signalRegion_NN_mh150}
\end{figure*}

\begin{figure*}[!h] 
 \centering 
 \subfloat[]{
  \includegraphics[width=0.32\textwidth]{fig/NN/NNout_Stacked_NormBillFit_mh180_jb0.png}
 }
 \subfloat[]{
  \includegraphics[width=0.32\textwidth]{fig/NN/NNout_Stacked_NormBillFit_mh180_jb1.png}
 }
 \subfloat[]{
  \includegraphics[width=0.32\textwidth]{fig/NN/NNout_Stacked_NormBillFit_mh180_jb2.png}
 }
\caption{NN output distributions of the signal region in the 165 -- 195 GeV mass region, 
 for which the NN was trained at 180 GeV. Subfigure (a) shows the distribution of the 0-jet channel, 
 (b) the distribution of the 1-jet channel and (c) the distribution of the 2-jet channel. 
 The distributions of simulated events are normalised to data.}
 \label{fig:signalRegion_NN_mh180}
\end{figure*}

\begin{figure*}[!h] 
 \centering 
 \subfloat[]{
  \includegraphics[width=0.32\textwidth]{fig/NN/NNout_Stacked_NormBillFit_mh300_jb0.png}
 }
 \subfloat[]{
  \includegraphics[width=0.32\textwidth]{fig/NN/NNout_Stacked_NormBillFit_mh300_jb1.png}
 }
 \subfloat[]{
  \includegraphics[width=0.32\textwidth]{fig/NN/NNout_Stacked_NormBillFit_mh300_jb2.png}
 }
\caption{NN output distributions of the signal region in the 260 -- 340 GeV mass region, 
 for which the NN was trained at 300 GeV. Subfigure (a) shows the distribution of the 0-jet channel, 
 (b) the distribution of the 1-jet channel and (c) the distribution of the 2-jet channel. 
 The distributions of simulated events are normalised to data.}
 \label{fig:signalRegion_NN_mh300}
\end{figure*}

\begin{figure*}[!h] 
 \centering 
 \subfloat[]{
  \includegraphics[width=0.32\textwidth]{fig/NN/NNout_Stacked_NormBillFit_mh400_jb0.png}
 }
 \subfloat[]{
  \includegraphics[width=0.32\textwidth]{fig/NN/NNout_Stacked_NormBillFit_mh400_jb1.png}
 }
 \subfloat[]{
  \includegraphics[width=0.32\textwidth]{fig/NN/NNout_Stacked_NormBillFit_mh400_jb2.png}
 }
\caption{NN output distributions of the signal region in the 360 -- 440 GeV,
 for which the NN was trained at 400 GeV. Subfigure (a) shows the distribution of the 0-jet channel, 
 (b) the distribution of the 1-jet channel and (c) the distribution of the 2-jet channel. 
 The distributions of simulated events are normalised to data.}
 \label{fig:signalRegion_NN_mh400}
\end{figure*}

\begin{figure*}[!h] 
 \centering 
 \subfloat[]{
  \includegraphics[width=0.32\textwidth]{fig/NN/NNout_Stacked_NormBillFit_mh600_jb0.png}
 }
 \subfloat[]{
  \includegraphics[width=0.32\textwidth]{fig/NN/NNout_Stacked_NormBillFit_mh600_jb1.png}
 }
 \subfloat[]{
  \includegraphics[width=0.32\textwidth]{fig/NN/NNout_Stacked_NormBillFit_mh600_jb2.png}
 }
\caption{NN output distributions of the signal region in the 560 -- 640 GeV,
 for which the NN was trained at 600 GeV. Subfigure (a) shows the distribution of the 0-jet channel, 
 (b) the distribution of the 1-jet channel and (c) the distribution of the 2-jet channel. 
 The distributions of simulated events are normalised to data.}
 \label{fig:signalRegion_NN_mh600}
\end{figure*}
